# Supplementary material for: Learning with Multi-modal Gradient Attention for Explainable Composed Image Retrieval
Source: arXiv:2308.16649 source file (2023-08-31)
Supplement: Supplementary file 1 [file Supp_fig_FashionIQ.pdf]

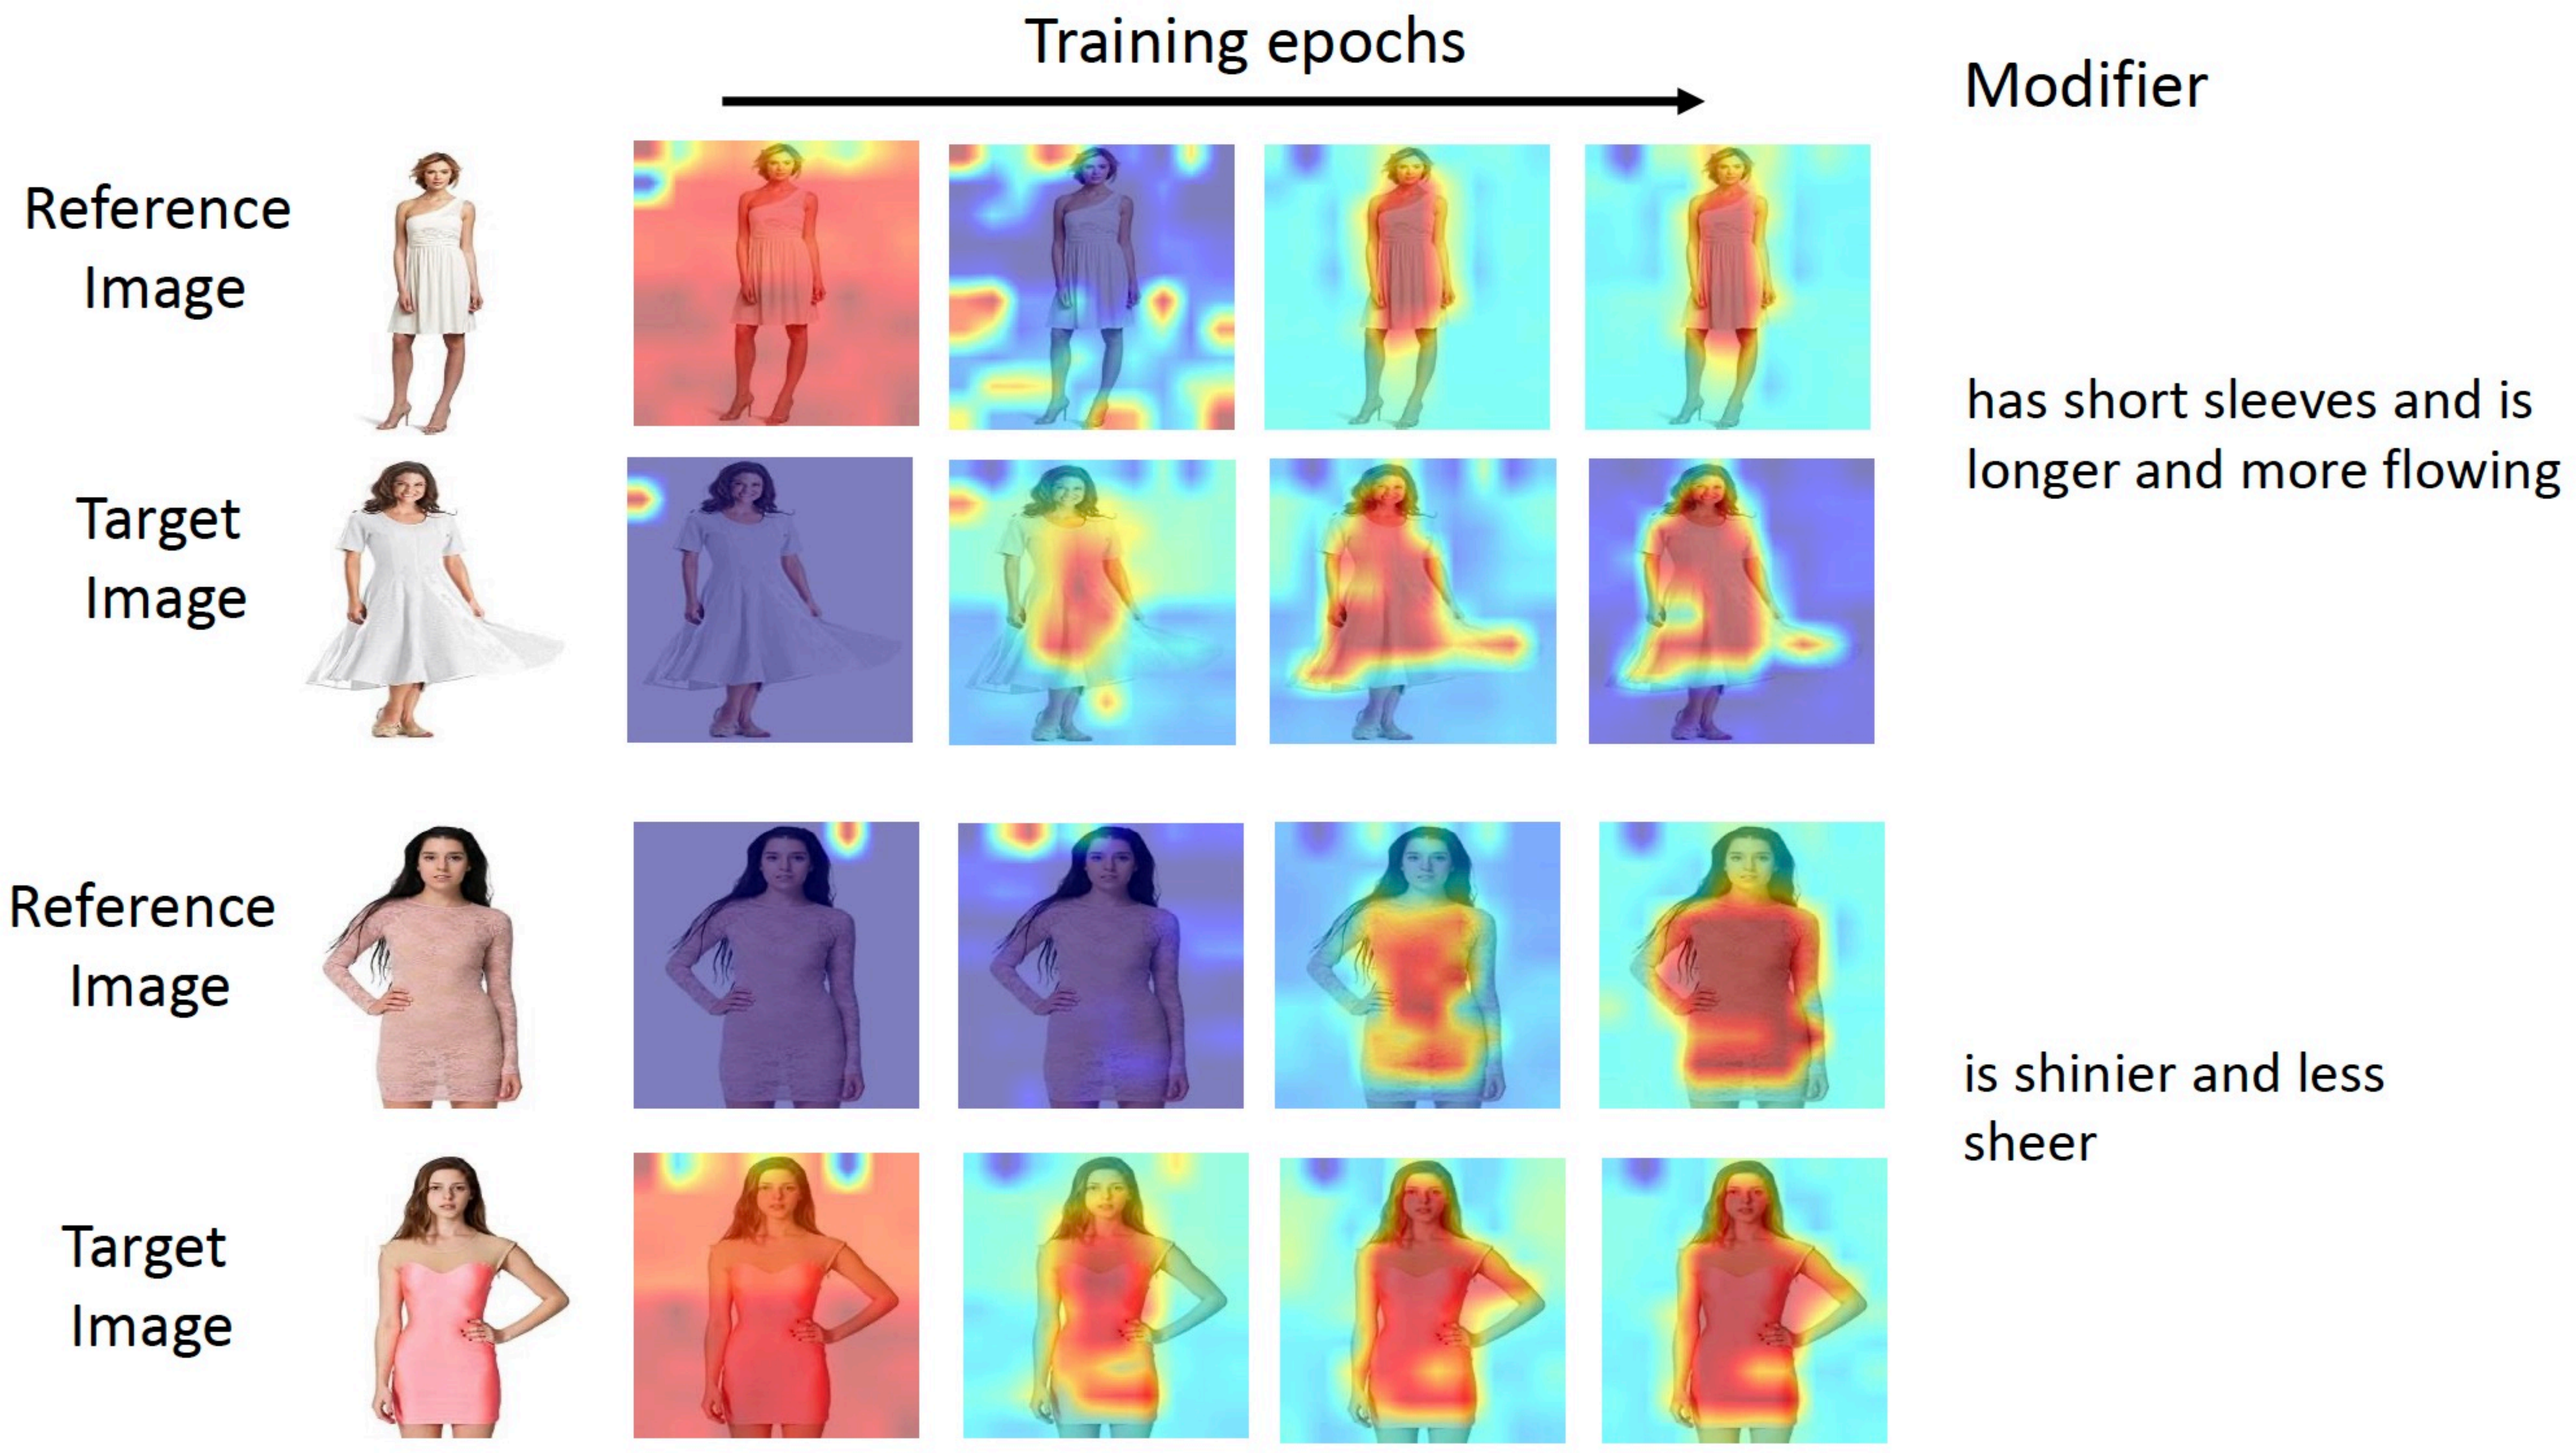
Training epochs
Modifier
Reference Image
Target Image
has short sleeves and is longer and more flowing
Reference Image
Target Image
is shinier and less sheer

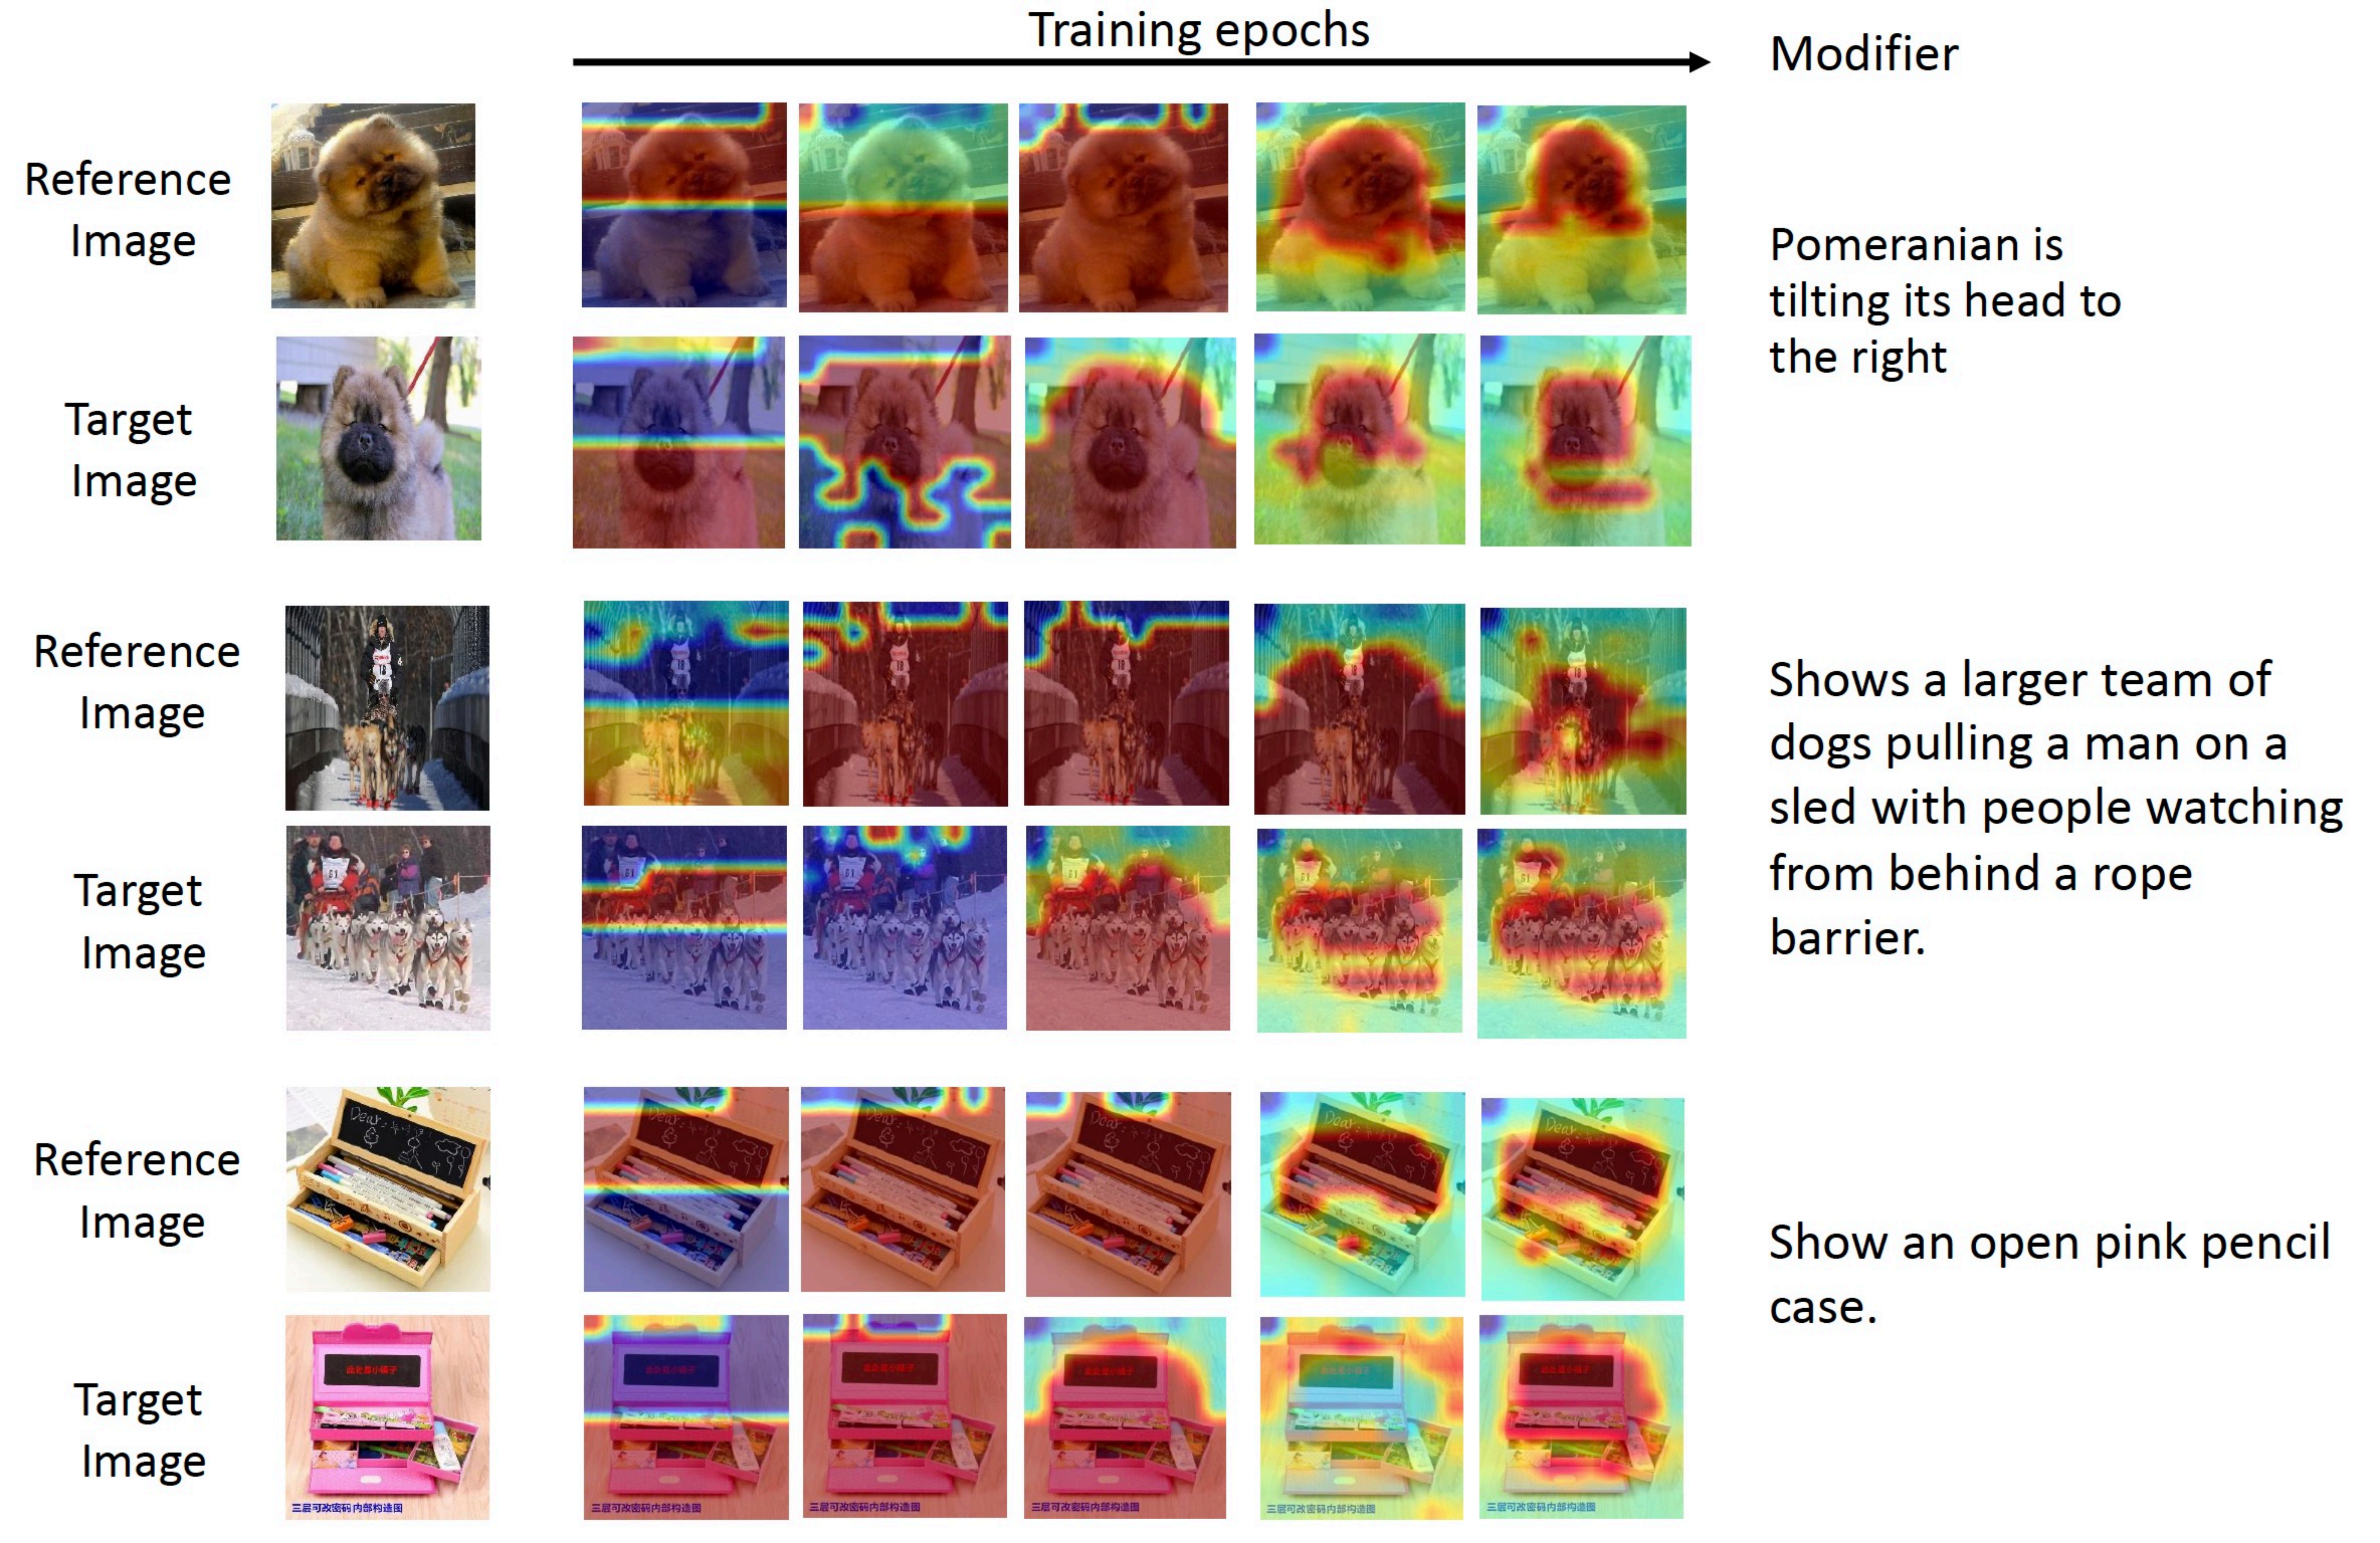
Training epochs
Modifier
Reference Image
Target Image
Pomeranian is tilting its head to the right
Reference Image
Target Image
Shows a larger team of dogs pulling a man on a sled with people watching from behind a rope barrier.
Reference Image
Target Image
Show an open pink pencil case.

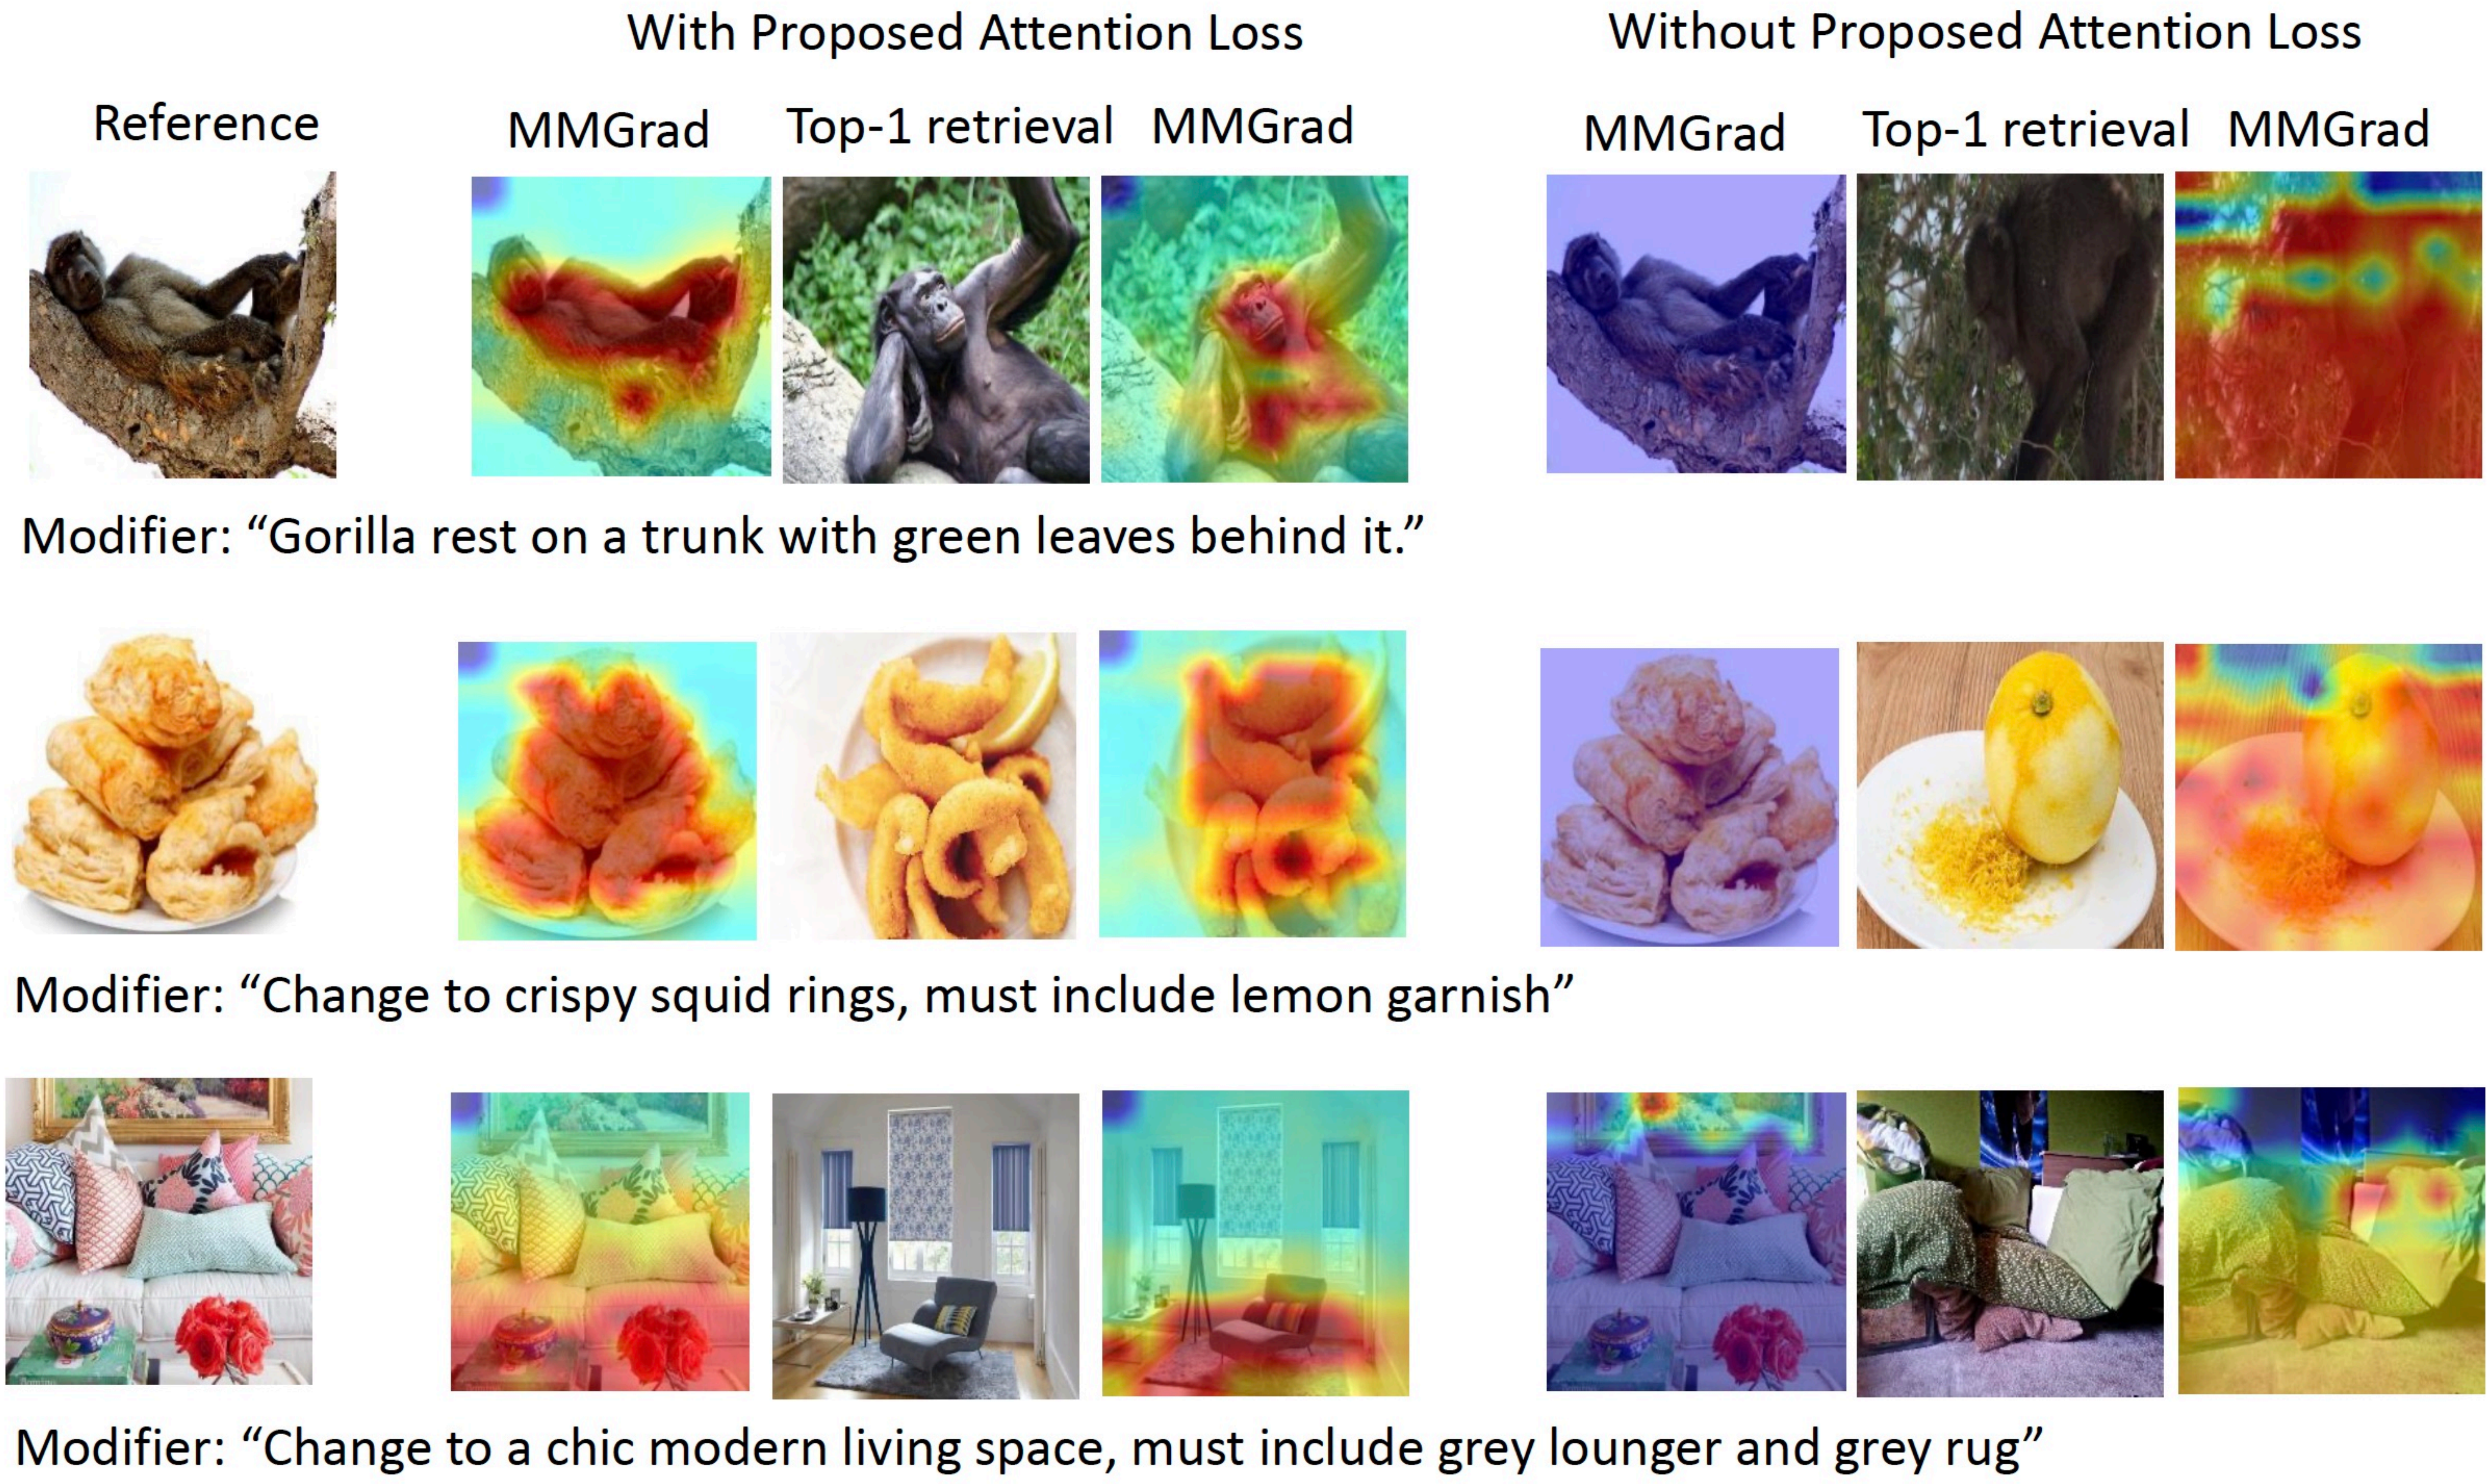
With Proposed Attention Loss
Without Proposed Attention Loss
Reference
MMGrad
Top-1 retrieval
MMGrad
MMGrad
Top-1 retrieval
MMGrad
Modifier: "Gorilla rest on a trunk with green leaves behind it."
Modifier: "Change to crispy squid rings, must include lemon garnish"
Modifier: "Change to a chic modern living space, must include grey lounger and grey rug"

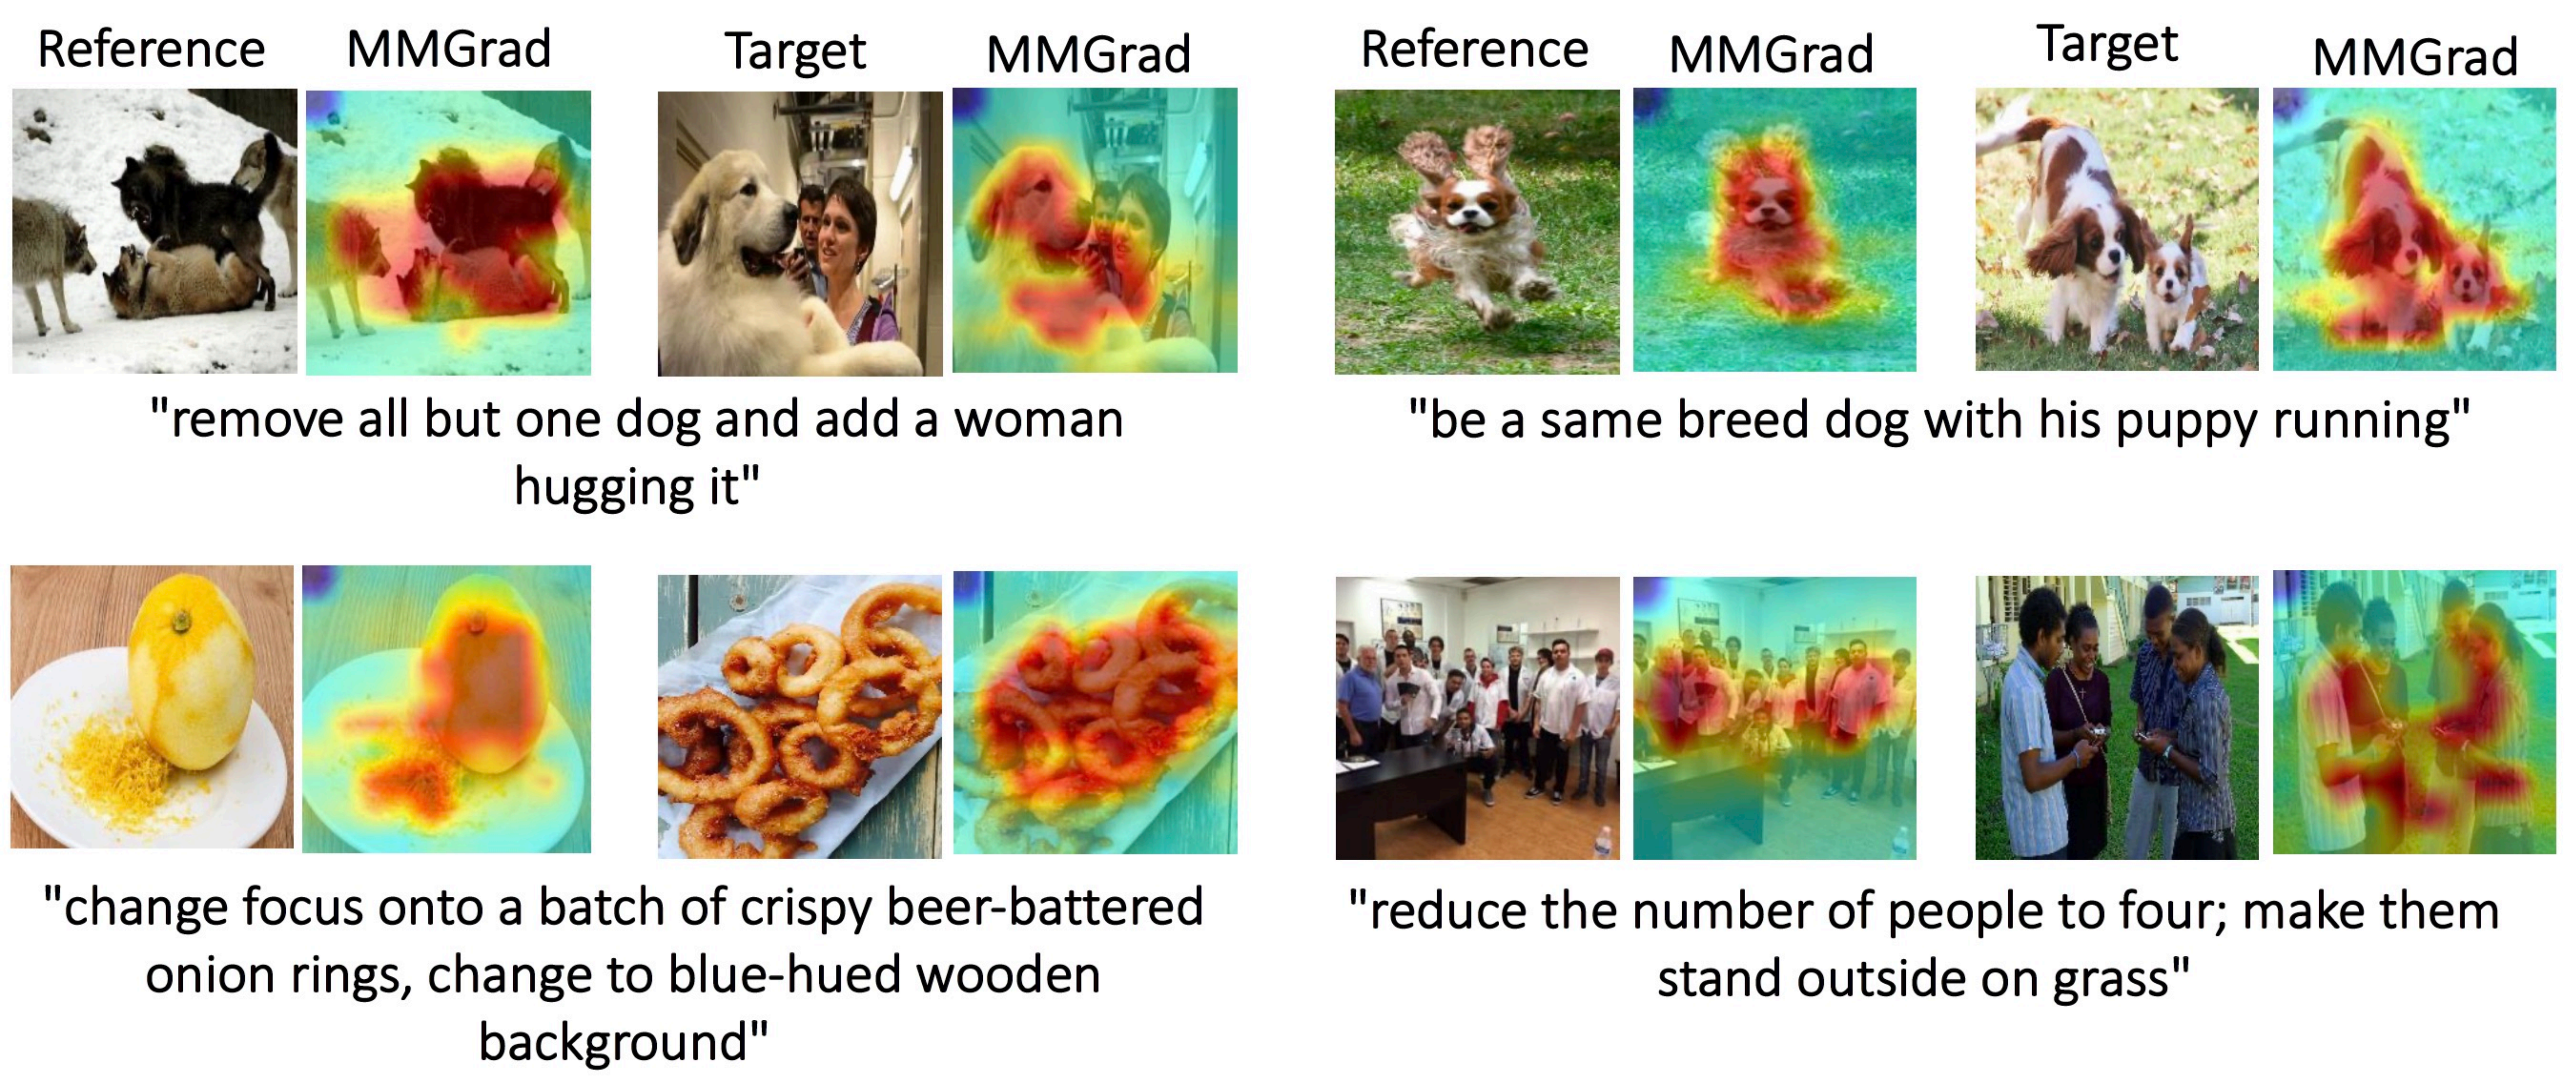
Reference
MMGrad
Target
MMGrad
"remove all but one dog and add a woman hugging it"
Reference
MMGrad
Target
MMGrad
"be a same breed dog with his puppy running"
"change focus onto a batch of crispy beer-battered onion rings, change to blue-hued wooden background"
"reduce the number of people to four; make them stand outside on grass"
